# Supplementary material for: Bounding the Distance to Unsafe Sets with Convex Optimization
Source: arXiv:2110.14047 source file (2023-03-09)
Supplement: Supplementary file 1 [file appendix_duality.tex]

% \appendix
\appendices
\section{Proof of Strong Duality in Theorem \ref{thm:strong_duality_dist}}
\label{app:duality}
This proof will follow the method used in the proof of Theorem 2 in \cite{henrion2013convex} to prove duality. The first step will prove that programs \eqref{eq:dist_meas} and \eqref{eq:dist_cont} are (weakly) dual to each other, and the next step will prove that strong duality holds.

The two programs will be posed as a pair of standard-form infinite dimensional 
LPs.
The following spaces may be defined:
\begin{align}
    \mathcal{C} &= C(X_0) \times C([0, T]\times X)^2 \times C(X \times X_u) \label{eq:dual_spaces}\\
    \mathcal{Q} &= \mathcal{M}(X_0) \times \mathcal{M}([0, T]\times X)^2 \times \mathcal{M}(X \times X_u). \nonumber
\end{align}
The nonnegative subcones of $\mathcal{C}$ and $\mathcal{Q}$ respectively are,
\begin{align}
    \ks &= C_+(X_0) \times C_+([0, T]\times X)^2 \times C_+(X \times X_u) \label{eq:dual_cones}\\
    \ks' &= \Mp{X_0} \times \Mp{[0, T]\times X}^2 \times \Mp{X \times X_u}. \nonumber
\end{align}

The cones $\ks$ and $\ks$ in \eqref{eq:dual_cones} are topological duals, and the measures from \eqref{eq:dist_meas_joint}-\eqref{eq:dist_meas_init} satisfy $\psi = (\mu_0, \mu_p, \mu, \eta) \in \ks'$.

The spaces $\mathcal{P}$ and $\mathcal{R}$ may be defined as,
\begin{align}
    \mathcal{P} &= C(X) \times C^1([0, T] \times X) \times \R \\
    \mathcal{R} &= \mathcal{M}(X) \times C^1([0, T] \times X)' \times \R.
\end{align}
The arguments $z = (w, v, \gamma)$ from problem \eqref{eq:dist_cont} are members of the set $\mathcal{P}$.
The linear operators $\A': \ks' \rightarrow \mathcal{R}$ and $\A: \mathcal{P} \rightarrow \mathcal{C}$ induced from constraints \eqref{eq:dist_meas_marg}-\eqref{eq:dist_meas_prob} may be defined as,
\begin{align}
    \A'(\psi) =[&\pi^{x}_\# \mu_p -\pi^{x}_\# \eta, \delta_0 \otimes\mu_0 + \Lie_f^\dagger \mu - \mu_p, \inp{1}{\mu_0}]\nonumber\\ 
    \A(z) = [&v(0,x)-\gamma, w(x)-v(t,x), \Lie_f v(t,x), \\
    &c(x,y)-w(x)].\nonumber
\end{align}

The last pieces needed to convert \eqref{eq:dist_meas} into a standard-form LP are the cost vector $\ell = [0, 0, 0, c(x, y)]$ and the answer vector $\beta = [0, 0, 1] \in \mathcal{R}$. Problem \eqref{eq:dist_meas} is therefore equivalent to (with $\inp{\ell}{\psi} = \inp{c}{\eta}$),
\begin{align}
    p^* =& \min_{\psi \in \ks'} \inp{\ell}{\psi} & & \A'(\psi) = \beta. \label{eq:dist_meas_std}\\
\intertext{The dual LP to \eqref{eq:dist_meas_std} in standard form is (with $\inp{\beta}{z} = \gamma$),}
    d^* = &\max_{z \in \mathcal{P}} \inp{\beta}{z}
    & &\A(z) - \ell \in \ks. \label{eq:dist_cont_std}
\end{align}

The operators $\A$ and $\A'$ are adjoints with $\inp{\A(z)}{\psi} = \inp{z}{\A'(\psi)}$ for all $z \in \mathcal{C}$ and $\psi \in \ks'$. Program \eqref{eq:dist_cont_std} is equivalent to program \eqref{eq:dist_cont}, therefore proving (weak) duality of programs \eqref{eq:dist_meas} and \eqref{eq:dist_cont} (proposition C.19 of \cite{lasserre2009moments}).

Strong duality between \eqref{eq:dist_meas} and \eqref{eq:dist_cont} $(p^* = d^*)$ holds if the image of the affine map $\mathcal{I} = \{(\A'(\psi), \inp{\ell}{\psi}) \mid \psi \in \ks'\}$ is closed in the weak-* topology and if $p^*$ is bounded below by Theorem 3.10 of \cite{anderson1987linear}. The function $c(x, y)$ has a minimal value of $0$ when $x = y \in X_u$, so $p^*$ has a finite lower bound of $0$. 
The mapping $\A'(\psi)$ is weak-* continuous because $\forall z \in \mathcal{P}: \A(z) \in \mathcal{C}$ (refer to footnote 10 of \cite{henrion2013convex} for more detail).
Let $\{\psi_k\}$ be a \rev{sub}sequence in $\ks'$ that converges to $\lim_{k\rightarrow \infty} \psi_k = \psi$ \rev{with} $(\nu, \alpha) = \lim_{k\rightarrow \infty}(\A'(\psi_k), \inp{\ell}{\psi_k})$. 
Closure of $\mathcal{I}$ in the weak-* topology requires that the accumulation point $(\nu, \alpha) $ of every \rev{sub}sequence $\{\psi_k\}$ is inside $\mathcal{I}$. 

% Define the test functions $\xi_j$ for $j=1, \ldots, 4$ and perform pairings $\inp{\xi_j}{\A'(\psi_k)} \rightarrow \inp{\xi_j}{\nu}$, 
% \begin{align*}
%     \xi_1&= (0, 0, 1):  & \inp{1}{\mu_{0k}} \rightarrow \inp{\xi_1}{\nu} &
%     < \infty \\
%     \xi_2 &= (0, -1, 1):  & \inp{1}{\mu_{pk}} \rightarrow \inp{\xi_2}{\nu} &< \infty \\
%     \xi_3 &= (-1, -1, 1): & \inp{1}{\eta_k} \rightarrow \inp{\xi_3}{\nu} &< \infty \\
%     \xi_4 &= (0, t-T, T): & \inp{1}{\mu_k} + \inp{T-t}{\mu_{pk}} \rightarrow \inp{\xi_4}{\nu} &< \infty.
% \end{align*}
% The masses of all measures are nonnegative (bounded below by 0), and are therefore bounded above by the restrictions in $\xi$.
% The evaluation $\inp{T-t}{\mu_{pk}}$ is nonnegative given that $\inp{1}{\mu_{pk}}$ is nonnegative and $\mu_{pk}$ is supported in time for $t \in [0, T]$. 

\rev{
We note that the masses of $\psi_k$ are bounded by Lemma \ref{lem:bounded}.
Let the notation $\weak$ denote convergence in the weak-* topology. If the subsequence $\{\psi_k\}$ converges weakly as $\psi_k \weak \psi$ in $\ks'$, then $\inp{\ell}{\psi_i} \rightarrow \inp{\ell}{\psi}$ for all $\ell \in \ks$ (definition of weak-* convergence). The set $\inp{\xi}{\A'(\psi_i)} \rightarrow \inp{\xi}{\A'(\psi)}, \forall \xi \in \mathcal{P}$, which holds because,
\begin{equation}
\label{eq:weak_a}
    \inp{\xi}{\A'(\psi_i)} = \inp{\A(\xi)}{\psi_i} \overset{\ast}{\rightharpoonup} \inp{\A(\xi)}{\psi} = \inp{\xi}{\A'(\psi)}.
\end{equation}
An equivalent statement to \eqref{eq:weak_a} is that $\A'(\psi_i) \overset{\ast}{\rightharpoonup} \A'(\psi)$ in $\mathcal{R}$, which demonstrates weak-* closedness. 
}
% \rev{Weak-* closedness of $\{\A'(\psi), \inp{\ell}{\psi}: \psi \in \ks' \subset \mathcal{R} \times \R\}$) may be proven.

% } 

% However, it seems to me that the (sequential) weak-* closedness of the set $\{\A'(\psi), \inp{\ell}{\psi}: \psi \in \ks' \subset \mathcal{R} \times \R\}$) can be proven using
% only the definition of weak-* convergence. Indeed, if $\psi_i \overset{\ast}{\rightharpoonup} $ in $\ks'$, then by definition
% of weak-* convergence $\inp{\ell}{\psi_i} \rightarrow \inp{\ell}{\psi}$, so there remains to show that $\A'(\psi_i) \overset{\ast}{\rightharpoonup} \A'(\psi)$ in $\mathcal{R}$. This is equivalent to showing that $\inp{\xi}{\A'(\psi_i)} \rightarrow \inp{\xi}{\A'(\psi)}$ for every $\xi \in \mathcal{P}$, which
% is true because
% \begin{equation*}
%     \inp{\xi}{\A'(\psi_i)} = \inp{\A(\xi)}{\psi_i} \overset{\ast}{\rightharpoonup} \inp{\A(\xi)}{\psi} = \inp{\xi}{\A'(\psi)},
% \end{equation*}
% Passage to the limit is warranted once again by the definition of weak-* convergence.

% The weak-* compactness of the unit ball by Alaoglu's theorem may be used to find a convergent subsequence $\{\xi_{i}\}$ of $\{\xi_k\}$ such that $\lim_{i \rightarrow \infty} (\A'(\psi_i), \inp{\ell}{\psi_i}) \rightarrow (\nu, \alpha)$. 
Conditions for strong duality have now been met, proving that the objectives of \eqref{eq:dist_meas} and \eqref{eq:dist_cont} are equal under assumptions A1-A5.
